# Supplementary material for: Leveraging Randomized Smoothing for Optimal Control of Nonsmooth Dynamical Systems
Source: arXiv:2203.03986 source file (2024-01-22)
Supplement: Supplementary file 1 [file appendix.tex]

\section*{Appendix}

\subsection{Evolution strategies from the Randomized Smoothing point of view} \label{sec:ES_RS}

Evolution Strategies (ES)\cite{salimans2017evolution,mania2018simple} are algorithms aiming at minimizing \eqref{uncons_policyRL} but that use as descent directions, gradients different from RL:
\begin{align}
    \nabla_\theta R_{ES} &= \mathbb{E}_\zeta \left[ R(x(\theta, \zeta),u(\theta, \zeta))  \nabla_\theta \log p_\theta(\zeta) \right] \label{eq:grad_ES}
\end{align}
where stochasticity is introduced in these strategies directly at the parameter levels \eqref{eq:grad_ES}. Thus, ES use a deterministic policy but parameterize it with a stochastic parameter.
 
\subsection{Randomly smoothed gradient descent to solve optimal control with non-smooth dynamics }
\ql{Remove this subsection as it indicates potential future line of work ? }
\begin{align}
    \min_{u}& \ R(x^\epsilon(u),u)    \label{smooth_OC}
\end{align}
where:
\begin{align}
    x^\epsilon_{t+1}(u) &= f_\epsilon(x^\epsilon_t,u_t),\\
    x_0 = \overline{x_0}\end{align}
and $ f_\epsilon(x,u) = \mathbb{E}_U\left[f(x,u+\epsilon U)\right]$ is a smooth approximation of the dynamic. In practice, $\Tilde{f}$ is approximated with a Monte Carlo estimator by running several simulation in parallel. 

With this approach, several samples are averaged after each time step which allows to smooth the dynamics. Doing so also limits the diffusion of the noise and reduces the amount of exploration. Thus, in order to increase the exploration of the algorithm, a possibility consists in averaging at the end of the whole trajectory. This can be written:

\begin{align}
    \min_{u}& \  R(\hat{x}(u),u)    \label{smooth_OC2}
\end{align}
where:
\begin{align}
    \hat{x}_1(u) &= \mathbb{E}_U[{f}(x_0,u_0 + \epsilon U_0)],\\
    \hat{x}_2(u) &=  \mathbb{E}_U[{f}({f}(x_0,u_0 + \epsilon U_0),u_1 + \epsilon U_1)],\\
    &\vdots \\
    \hat{x}_T(u) &= \mathbb{E}_U[f(...f(x_0,u_0 + \epsilon U_0)u_1+ \epsilon U_1),...u_{T-1} + \epsilon U_{T-1}),u_T + \epsilon U_T)]
\end{align}
and it appears that the recursivity of the problem is lost which makes it impossible to exploit the Bellman equation to solve it efficiently as done in DDP. 

An intermediate solution which allows to retrieve the recursive property consists in averaging after a fixed number $k$ of steps. For instance, taking $k=2$ gives:

\begin{align}
    \min_{x,u}& \ R(x,u)\\
    s.t. &  \ \forall t \in \left[1,\lfloor(T-1)/2\rfloor \right], \ x_{t+2} = \Tilde{f}(x_t,u_t,u_{t+1}),  \\
    & x_0 = x(0)
\end{align}
where $f_\epsilon(x_t,u_t,u_{t+1}) = \mathbb{E}_U \left [  f( f(x_t,u_t + \epsilon U_t),u_{t+1} + \epsilon U_{t+1}) \right ]$ corresponds to the smoothed version of $f$ composed k times. This remains valid for dynamics defined implicitly.

\subsection{Random Search is Randomized Smoothing for policy learning}

Because the model of the dynamic $f$ can be stochastic or an approximation of the true dynamics, rather than an optimal trajectory $\tau = (x,u)$, one should look for a policy $\pi :  \mathcal{S} \xrightarrow{} \mathcal{A}$, providing an action as a function of a feedback on the state (An other possibility would be to use a state feedback and re-compute online the new optimal trajectory with the current state as initialization, this method corresponds to Model Predictive Control (MPC) and the induced computation can make it difficult to run in real-time).

Following \cite{recht2019tour}, the problem can be written:

\begin{align}
  \min_{x,u,\pi}& \ R(x,u)   \\
  s.t. &  \ \forall t \in \left[1,T-1\right], \ x_{t+1} = f(x_t,u_t), \\
 &  \ \forall t \in \left[1,T-1\right], \ u_t = \pi_t(x_t) \\
 & x_0 = \overline{x_0}
\end{align}

Due to the intractability of the problem of optimizing over the whole functional space, $\pi$ is usually restricted to a class of parameterized functions, and the problem we consider is:

\begin{align}
  \min_{x,u,\theta}& \ R(x,u)   \\
  s.t.  \  & x_{t+1} = f(x_t,u_t) \ \forall t \in \left[1,T-1\right],\\
 &    u_t = \pi_\theta(x_t) \ \forall t \in \left[1,T-1\right], \\
 & x_0 = \overline{x_0}.
\end{align}

\textbf{Remark :} As described previously, with a good initialization DDP allows to get the optimal trajectory. In addition, the algorithm also provide a linear policy of the form $\pi_t(x_t) = k_t + K_t x_t$ which is optimal in the neighborhood of the optimal trajectory $\tau$. For an infinite time horizon, the policy is stationary so $k_t$ and $k_t$ does not depend on $t$ anymore.

To solve this new problem, we can proceed in a way similar to \eqref{uncons_OC} and substitute the variables $x,u$ by using the constraints :

\begin{align}
    \min_{\theta}& \  \Tilde{R}(\theta) = R(x(\theta),u(\theta))    \label{uncons_policy}
\end{align}

where:
\begin{align}
    x_{t+1}(\theta) &= f(x_t,\pi_\theta(x_t)),\\
    x_0(\theta) = \overline{x_0}
\end{align}

Solving this problem with a "gradient descent"-like algorithm would lead to a local solution and we detailed in \ref{sec:local_OC} why it can be problematic. In an alternative approach, \cite{mania2018simple} uses  random search over $\theta = (k,K)$ to optimize a linear policy of the form $\pi_\theta(x) = k + Kx$. (equivalent to applying randomized smoothing to DDP  or \eqref{uncons_OC}?)
The random optimization process is as follows:

\begin{align}
    \theta_{i+1} = \theta_i - \alpha \frac{\Tilde{R}(\theta_i + \delta \Theta)-\Tilde{R}(\theta_i - \delta \Theta)}{2 \delta} \Theta
\end{align}
where $\Theta \approx \mathcal{G}(0,1)$

This process can be interpreted as performing a stochastic gradient descent on $\hat{R}$, a randomly smoothed approximation of the objective function $\Tilde{R}$ (\cite{NEURIPS2020_6bb56208}, \cite{nesterov2017random}):
\begin{align}
    \mathbb{E}_\Theta \left[ \frac{\Tilde{R}(\theta + \delta \Theta) - \Tilde{R}(\theta - \delta \Theta)}{2 \delta} \Theta \right] &= \nabla_\theta \mathbb{E}_\Theta \left[ \Tilde{R}(\theta + \delta\Theta) \right] \\
    &= \nabla_\theta \hat{R}(\theta) \label{smooth_RS}
\end{align}
By substituting both the state and control variables, this approach leads to an unconstrained optimization problem but does not exploit the specific structure of the original problem. This allows to get a cost function implicitly containing the dynamics and which makes it possible to optimize $\Tilde{R}$ in a "black-box" way. For this reason, this algorithm is not competitive with DDP in terms of sample efficiency (random search is at most n times slower than classical gradient descent as shown in \cite{nesterov2017random}). However, doing so they avoid non-smoothness or non-convexity issues from the dynamics or the reward functions which are both smoothed by the randomization. \cite{mania2018simple} demonstrate that such an approach is competitive with Reinforcement Learning for complex tasks on Mujoco benchmarks.
